# Supplementary material for: L-Violating Supersymmetry - Implementation in PYTHIA and study of LHC discovery potential
Source: arXiv:hep-ph/0108207 source file (2001-08-24)
Supplement: Supplementary file 1 [file neural.tex]

\section{Neural Network Learning Rules\label{app:neural}}
The neural networks employed in this work all learn by adjusting their
synaptic weights, temperatures, and biases at the end of each pass over the
learning samples in the direction which minimizes the error. This aprroach is
known as the \emph{gradient descent} method \cite{mcclelland89}. As the name
implies, the learning rule is defined by taking a step in weight space in the
direction of the gradient of the (squared) error:
\begin{equation}
p \to p + \Delta p = - \alpha\frac{\partial e^2}{\partial p} = p + 2\alpha e
\frac{\partial \mathcal{O}}{\partial p}
\end{equation} 
where $p$ represents any of the variable parameters in the network, 
$e=t-\mathcal{O}$ is the error on the output (target output: $t$, obtained
output: $\mathcal{O}$), and $\alpha$ is a learning
rate parameter. This rule does not necessarily have to be applied after every
event in the learning sample. In order to wash out sharp, irregular 
changes called for from
extreme events in the distributions, 
we do better in accumulating the parameter changes over some processing
period without invoking them. After the period, the \emph{accumulated} change to each
parameter is invoked, and the accumulated error is reset. 
In order to get as little statistical noise in
the parameter changes as possible, the period is set to be the number of
events in the learning sample. Denoting event number by $n$,
the learning rule above becomes:
\begin{equation}
p \to p + \Delta p = p + 2\alpha \sum_ne(n)
\frac{\partial \mathcal{O}(n)}{\partial p}
\end{equation} 
One further improvement can be made on the learning rule. Seeing as two
successive changes to the parameters of the network 
often go in roughly the same direction in parameter
space, something which often increases the learning speed of the network:
\begin{equation}
p \to p + \Delta p = p + 2\alpha \sum_ne(n)
\frac{\partial \mathcal{O}(n)}{\partial p} + \beta \Delta p^{\mathrm{last}}
\label{eq:learnrule}
\end{equation} 
where $\Delta p^{\mathrm{last}}$ is the change which was made the previous
period, and $\beta<1$ specifies the ``inertia'' of the system. 
We are now ready to specify the learning rules for each of the parameters of
the network in fig.~\ref{fig:netlayout}. 
These can be easily derived. 
\begin{eqnarray}
\frac{\partial \mathcal{O}}{\partial o_j} 
& = & \frac{H_j}{N_{\mathrm{hid}}} \\
\frac{\partial \mathcal{O}}{\partial w_{ij}} & = & \frac{o_j}{N_{\mathrm{hid}}} 
H_j(1-H_j)I_i \\
\frac{\partial \mathcal{O}}{\partial \epsilon_j} & = & o_jH_j(H_j-1)\\
\frac{\partial \mathcal{O}}{\partial \delta_i} & = &
\frac{I_i(1-I_i)}{T_i}\sum_j o_jH_j(H_j-1)w_{ij} \\
\frac{\partial \mathcal{O}}{\partial T_i} & = &
\frac{\mathrm{In}_i}{T_i^2}I_i(1-I_i)\sum_jo_jH_j(H_j-1)w_{ij}
\end{eqnarray}
Replacing these quantities back into eq.~(\ref{eq:learnrule}) directly 
yields the required learning rules.
